# Supplementary material for: Polarons shape the interlayer exciton emission of MoSe$_2$/WSe$_2$ heterobilayers
Source: arXiv:2407.15649 source file (2024-07-22)

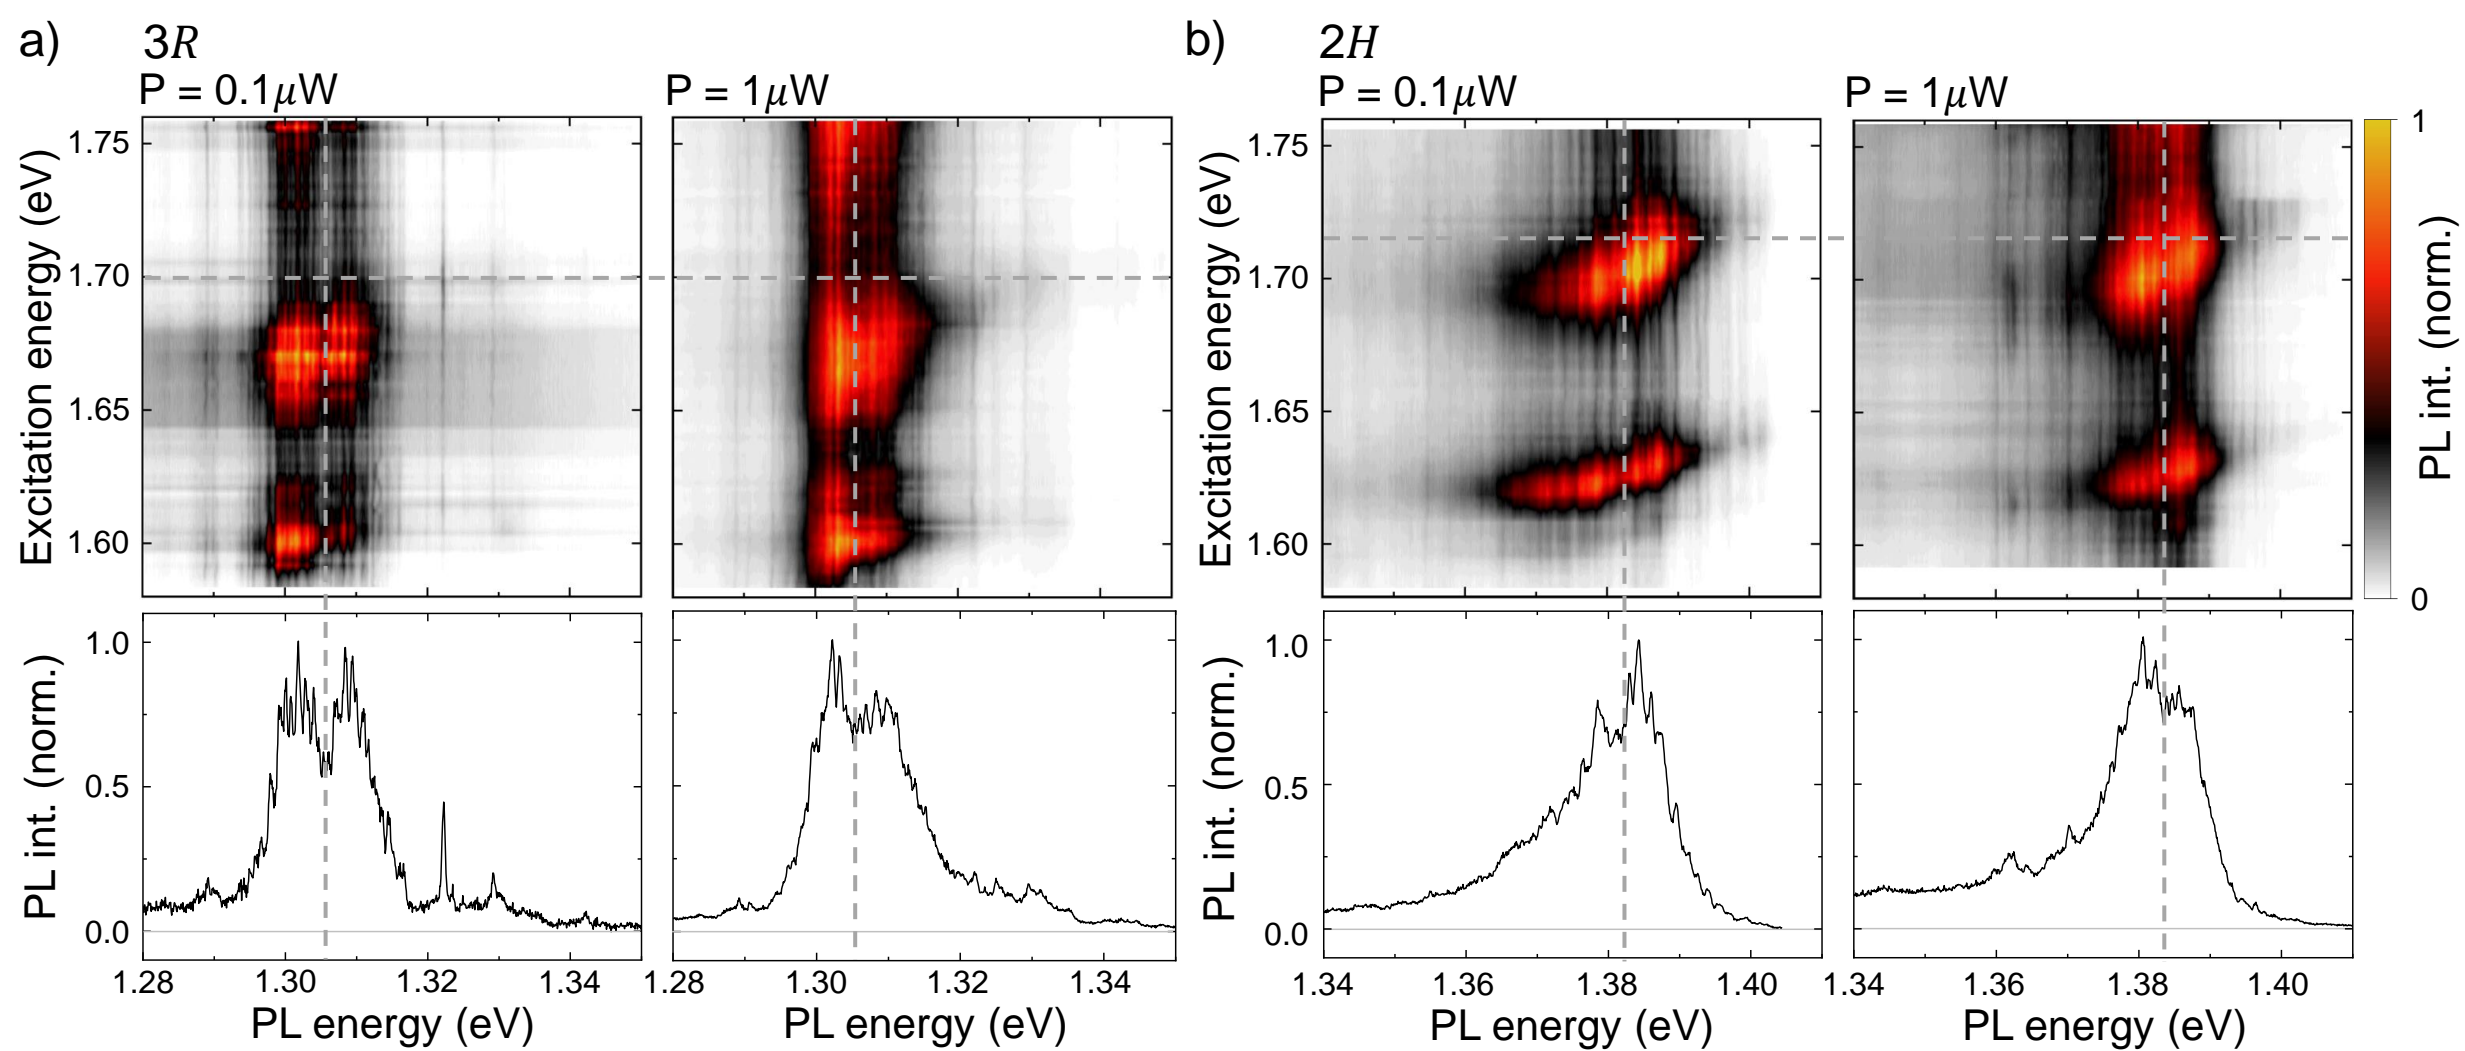

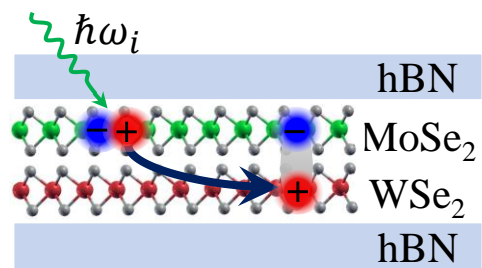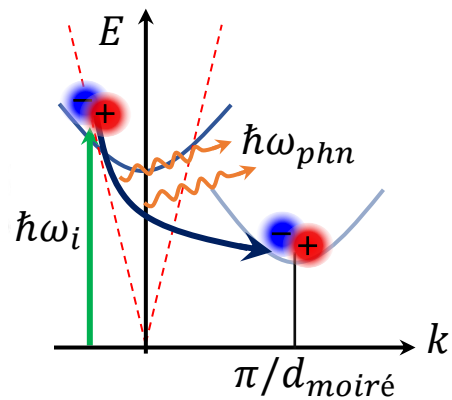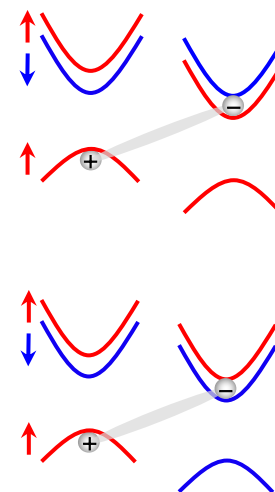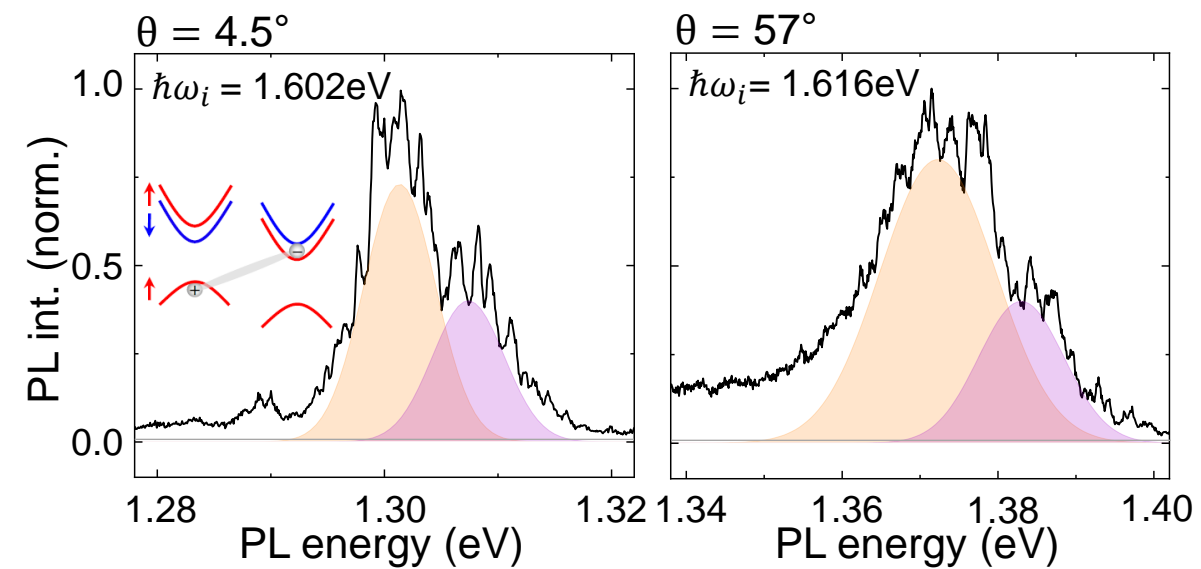

Supplement: Supplementary file 1 [file SM-3.pdf]
